# Supplementary material for: Ambipolar surface state transport in non-metallic stoichiometric Bi$_2$Se$_3$ crystals
Source: arXiv:1412.1422 source file (2015-07-20)
Supplement: Supplementary file 1 [file Bi2Se3_Insulating_PRX_SI.pdf]

# Supplemental Information: Ambipolar surface state transport in non-metallic stoichiometric $Bi_2Se_3$ crystals

Paul Syers[1] and Johnpierre Paglione[1,*]

[1]*Center for Nanophysics and Advanced Materials, Department of Physics, University of Maryland, College Park, MD 20742*

(Dated: July 20, 2015)

## A. Materials

In this section we provide further details of our experimental growth techniques. As stated in the main text, a pressurized gas furnace (Morris Research) was used in growing the samples of $Bi_2Se_3$ measured. Argon gas was used as the pressure medium in the furnace, which is capable of reaching pressures up to 200 bar at 1200°C. The gas was used to pump and flush the furnace chamber, before being sealed off at a controlled pressure before the start of the heating cycle. The pressure of the furnace chamber was continuously monitored during the growth cycle and it was determined that a room temperature pressure of roughly 45 bar consistently produces samples with the lowest carrier concentration. It should be noted that the growth tubes were laid in a nearly horizontal position in the furnace, with a slight vertical angle ($\leq$ 10°) and the measured carrier concentration varied monotonically with the part of the growth from which the sample was taken. Growths were heated at rate $\geq$50°C/h to 750°C, held for a few hours before being cooled at -20°C/h to 650°C, at which point the cooling rate was slowed down significantly and the growths were cooled further to 350°C before the furnace was turned off and allowed to cool at an uncontrolled rate. Quenching in water, from 450°C, was also tested on normal flux growth batches, but that only proved to greatly increase the bulk carrier concentration of the samples. It is assumed this is because at higher temperatures, the Se is much more mobile within the formed crystals, resulting in more Se vacancies, and quenching to room temperature effectively freezes in the higher defect density. Aside from time spent preparing the samples for measurements, all growths and samples were stored at room temperature under high vacuum.

## B. Measurements

We provide additional details in this section, pertaining to the behavior of the materials in the measurements discussed in this study. Electrical transport measurements were performed on all samples multiple times over a period of months. Measurements were made from 300 K to 1.8 K and up to ±14 T. A significant change in the temperature dependence between measurements taken two days apart was observed in some samples, a major sign of the volatility of the chemical potential in undoped $Bi_2Se_3$. Little ($\leq$ 10%) thermal cycling was seen in sample F during measurements, and none in all other samples. Later measurements taken on the nonmetallic samples a few months after the data shown in the main body of the paper did not show any of the non-metallic behavior in any of the samples. The top plot in Fig. 1 shows the change in resistivity for the samples over time and the two curves for sample A illustrate how rapidly the characteristics of this material can change between measurements taken only 2 days apart. While significant changes in sample quality due to exposure to air have been seen [1, 2], this is evidence that even storage at room temperatures in vaccuum is not enough to prevent such changes.

The longitudinal magnetoresistance (MR) of nearly all samples, shown in the bottom of Fig. 1, follows the strong, quasi-linear MR seen in previously reported low doped samples [3]. While the magnitude of the MR seems to have no correlation with carrier concentration or insulating behavior, Sample A stands out from the others due to its cusp-like behavior at low fields, and its non-linear behavior at high fields. The low field behavior resembles the weak antilocalization cusps previously reported in thin films of $Bi_2Se_3$ [4], however, fits to the expected WAL behavior fail to correctly describe the behavior.

Scanning electron microscopy and energy-dispersive electron spectroscopy (EDS) measurements were performed on all samples after all transport measurements, showing no sign of multiple phases, twinning, or any other large scale defects. Only signatures of Bi and Se were observed, and the ratios of constituent elements were within experimental error of stoichiometric ratios expected for $Bi_2Se_3$.

## C. Analysis

Here we present our method for obtaining curve fits to the Hall effect data, using a two band model [5], as well as our method for placement of the Fermi energies in bismuth selenide's band structure. The Hall resistance vs field data in Fig. 2 shows significant nonlinear behavior. The data was antisymmetrized, to isolate the $\rho_{xy}$ component. Even after antisymmetrization of the Hall effect data, samples A and F showed strong extreme curvature

*Electronic address: paglione@umd.edu

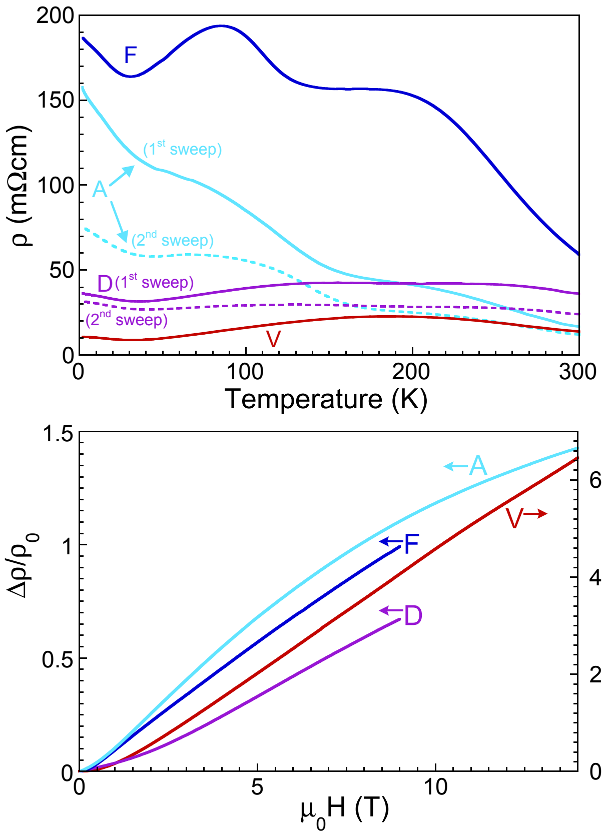


FIG. 1: (Top) Resistivity temperature dependence of four different samples of $Bi_2Se_3$, with some curves as indicated presenting a second data set measured using the same sample after a time delay (see text). (Bottom) Magnetoresistance of four different samples of $Bi_2Se_3$. The inset in the bottom graph shows the same data at low fields, highlighting the deviation from $H^2$ behavior in samples A and D.

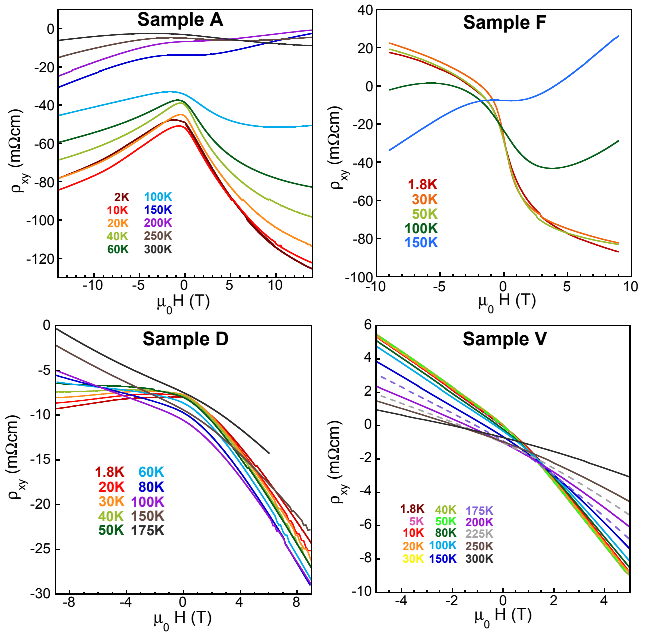


FIG. 2: Hall resistance vs magnetic field shown for all four samples discussed. Each plot shows all curves taken at different temperatures before applying anti-symmetrization analysis.

and a crossover in the sign of the Hall coefficient.

The following expression of the Drude model was used to fit the symmetrized Hall data

$$\rho_{xy} = \frac{{\sigma_h}^2 R_h - {\sigma_e}^2 R_e - {\sigma_h}^2 {\sigma_e}^2 R_h R_e (R_h - R_e) H^2}{(\sigma_h + \sigma_e)^2 + {\sigma_h}^2 {\sigma_e}^2 (R_h - R_e)^2 H^2} H \quad (1)$$

with $\sigma$ and R being the conductivities and Hall coefficients of the contributing carrier types - holes and electrons. Given the nearly isotropic, single band nature of the Fermi surface of $Bi_2Se_3$, the following approximations were applied to the model: $R_i = 1/\eta_i e$, $\mu_i = \sigma_i R_i$ with $\eta$, $\mu$ being the carrier concentrations and mobilities, respectively and the index $i$ denoting electrons or holes. Using these conversions, we arrive at an expression of the Drude model that depends directly on the carrier concentrations and mobilities of the two types of carriers:

$$\rho_{xy} = \frac{{\mu_h}^2 p - {\mu_e}^2 n - {\mu_h}^2 {\mu_e}^2 (p - n) H^2}{(p\mu_h + n\mu_e)^2 + {\mu_h}^2 {\mu_e}^2 (p - n)^2 H^2} \frac{H}{e} \quad (2)$$

with $n$ and $p$ being the electron and hole carrier concentrations and $e$ being the electron charge. This gives a five dimensional parameter space for any curve fitting program to explore. Fitting each curve to the model directly produced insufficient and unreliable fits. Fixing the concentration or mobility of one carrier type would help provide a more stable fit, however this introduces nontrivial assumptions about the system. Another analytical method, however, allows a reduction of the parameter space without such assumptions. Equation 2 is of the general form $y = (ax + bx^3)/(c + dx^2)$ which can be re-expressed as a 3rd order polynomial. The polynomial can be solved by a simplified method of least squares fitting: singular value decomposition (SVD). The eigenvectors of the SVD are 4 component vectors; the components corresponding to values of $a$, $b$, $c$, and $d$. The eigenvector with the eigenvalue closest to zero should contain the values of the coefficients that create the closest possible fit to the data that the Drude model can produce.

While this method provides accurate values of $a$, $b$, $c$, and $d$, it does not necessarily mean that the physical parameters of carrier concentrations mobilities are obtainable from the fit, but in this case, conversions can be made between the polynomial coefficients and $n$, $p$, $\mu_h$ and $\mu_e$. It is important to note that the vector containing $a$, $b$, $c$, and $d$ can be modified by a scalar without affecting the accuracy of the fit. Thus, it is not necessarily the individual values of a,b,c, and d but rather the relationships among the parameters that are accurate. This means that for the fits, there is a scalar $S$ that functions as the free parameter and changing $S$ will change the resulting calculations of $n$, $p$, $\mu_e$, and $\mu_h$. The resulting

parameters are expressed by the following equations.

$$\mu_e = \frac{\sqrt{dS} - aS\sqrt{e} + \sqrt{(\sqrt{dS} - aS\sqrt{e})^2 + 4cS\sqrt{\frac{bSe}{d}}}}{2\sqrt{ct}} \tag{3}$$

$$\mu_h = \frac{\sqrt{\frac{bSe}{d}}}{\mu_e} \tag{4}$$

$$n = \frac{\sqrt{\frac{cS}{e}}\mu_e - \sqrt{\frac{dS}{e}}}{\mu_e{}^2 + \sqrt{\frac{b^2Se}{d}}} \tag{5}$$

$$p = n + \frac{d}{be} \tag{6}$$

The parameter space of $S$ was explored and a region within these limits was found where all four parameters had reasonable values expected for $Bi_2Se_3$. The same value of $S$ was used when calculating physical parameters for all data on each sample, but the value of $S$ was allowed to differ from sample to sample. Fig. 3 shows the best obtained values for carrier concentrations and mobilities for all samples discussed. The error bars come from fits using different values of $S$.

Samples D and V do not show direct evidence of both positive and negative carriers. The small amount of curvature in the data from the two samples is away from the x-axis, not towards it, which is counter to the behavior one would expect from a system with holes and electrons. Thus the two carrier model was adjusted, by changing the sign of the variable $p$ to reflect two bands of the sampe carrier type. The same procedure of SVD and subsequent conversion was successful for the adjusted model. The adjusted model was more accurate in fitting the data from samples D and V than the original model had been. The results from the adjusted model are also shown in Fig. 3.

Samples V and H showed signs of Shubnikov de Haas (SdH) oscillations. The oscillations in sample H have been discussed in the main paper and the oscillations measured in sample V have been plotted in Fig. 4. Modeling of the oscillatory signal using the standard Lifschitz–Kosevich formulism, shown as the solid red line in Fig. 4, can accurately fit the data with only one signal. Shifting of the lowest Landau levels, due to spin orbit coupling [6] causes a change in the oscillation frequency at the highest fields, as seen in Fig. 4b). Early discrepancies between the single frequency model and the data from sample V were resolved when adjusting for this LL-shifting.

The FFT peak was measured to be approximately 19 Tesla, and factoring in the aforementioned LL-shift at higher fields, the actual frequency is closer to 18 T, which corresponds to $n \approx 4.3 \times 10^{17}$ cm$^{-3}$, matching $n_b$ given by the Drude model. The Dingle temperature given by the model fit corresponds to $\mu \approx 900$ cm$^2$/Vs, which is close to the value of $\mu_b$ from the Drude model. Such close agreement between the SdH oscillations and one band of the two carrier model is strong evidence that the analysis technique is accurate, yet the absence of oscillations from the other band is puzzling. The parameters obtained from the model are listed in Table I. It is important to note the significant difference in phases of the two oscillation signals. Our model of the oscillations fits equally well when setting the phases to exactly $\pi$ and 0, but it breaks down when the phases are set equal to each other.

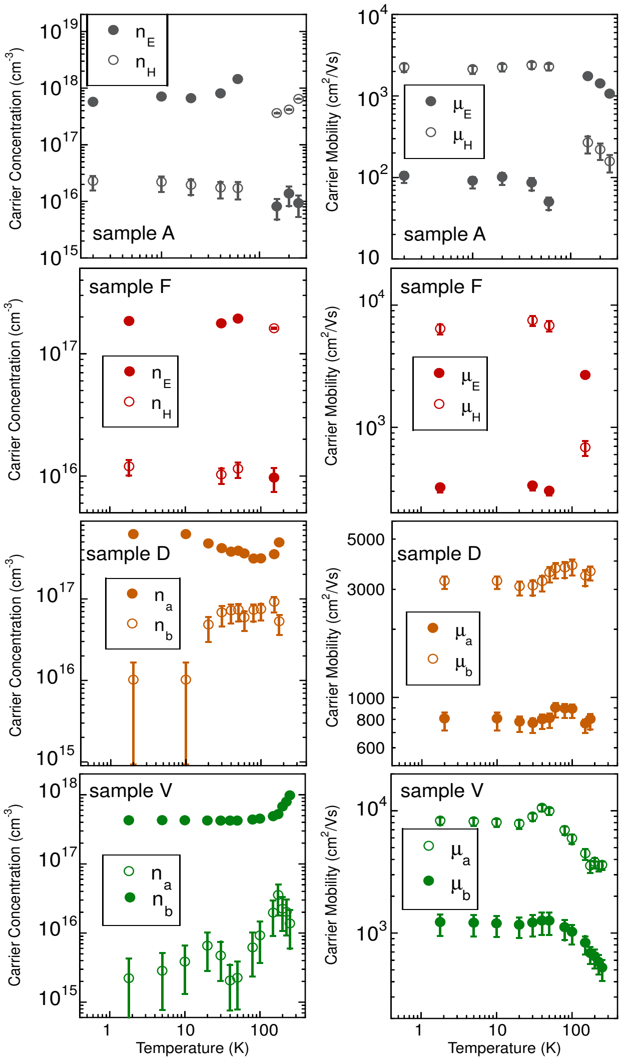


FIG. 3: Two-carrier analysis results yielding carrier concentration (left) and mobility (right) values in all four samples (see text).

While the surface band mobility calculated for sample H from the Dingle temperature is much lower than that given by the Drude analysis, the mobilities for the

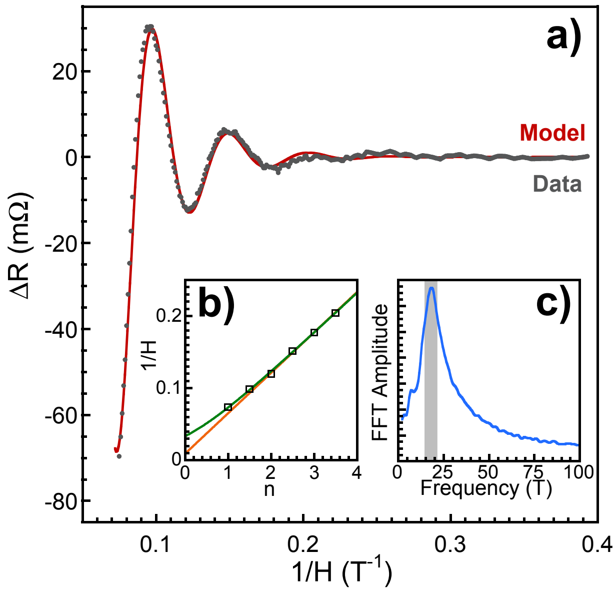


FIG. 4: Quantum oscillations of magnetoresistance of $Bi_2Se_3$ sample V, plotted as a function of inverse field. The solid red line is a fit to the oscillations using a single frequency model. The inset shows the Fourier Transform of the oscillations, with a single resonance peak indicating the low-frequency plotted in the main figure.

TABLE I: Physical Parameters extracted from Hall and SdH data on a high carrier concentration sample of $Bi_2Se_3$

| | Sample $H_a$ | Sample $H_b$ | Sample V |
|---|---|---|---|
| Drude $n$ ($\times 10^{18}$cm$^{-3}$) | 4.375 | 5.3 | 0.427 |
| Drude $\mu$ (cm$^2$/Vs) | 7,850 | 1,250 | 1,230 |
| SdH $n$ ($\times 10^{18}$cm$^{-3}$) | 4.4 | 5.3 | 0.424 |
| SdH $\mu$ (cm$^2$/Vs) | 2,660 | 1,970 | 1,130 |
| SdH $\phi$ (rad.) | 1.24$\pi$ | 0 | 0.534$\pi$ |

bulk band are relatively close in value for both samples H and V. Both analyses also show the expected behavior that the carriers at the surface have a higher mobility than those of the bulk. The close agreement of carrier concentrations, as well as the general agreement of mobilities of our two carrier model with the standard analysis method for the SdH oscillations measured in the same sample further confirms the model's validity.

For converting from $n$ to $k_f$, we used the following standard equation.

$$\textbf{3D:} k_f = (\frac{3N}{\pi})^{1/3} \tag{7}$$

We then used the band structure diagram for $Bi_2Se_3$-based on ARPES data by Bianchi et. al. [1] to estimate the location of $E_F$ for the surface and bulk states for each sample, given our calculated $k_F$ values and estimated carrier sign. The resultant diagram showing the placement of Fermi energies with respect to the conduction and valence bands is shown in Fig. 4 of the main paper. We use the equation for a 3D fermi space because all carrier concentrations calculated using the Drude model are expressed in cm$^{-3}$. Any geometric conversions of the concentrations attributed to the surface states would introduce unnecessary uncertainty. Given the orientation of the samples, the $k_f$ of the surface states would be at its maximum value, and therefore the accuracy of the estimates of $k_f$ would not be compromised.


[1] M. Bianchi, D. Guan, S. Bao, J. Mi, B. B. Iversen, P. D. C. King, and P. Hofmann, Nature Communications **1**, 128 (2010).

[2] R. V. Aguilar, L. Wu, A. V. S. an L S Bilbro, M. Brahlek, N. Bansal, S. Oh, and N. P. Armitage, Journal of Applied Physics **113**, 153702 (2013).

[3] N. P. Butch, K. Kirshenbaum, P. Syers, A. B. Sushkov, G. S. Jenkins, H. D. Drew, and J. Paglione, Physical Review B **81**, 241301 (2010).

[4] M. Bianchi, R. C. Hatch, D. Guan, T. Planke, J. Mi, B. B. Iversen, and P. Hofmann, Semiconductor Science and Technology **27**, 124001 (2012).

[5] R. G. Chambers, Proceedings of the Physical Society A **65**, 903 (1952).

[6] A. A. Taskin, Z. Ren, S. Sasaki, K. Segawa, and Y. Ando, Physical Review Letters **107**, 016801 (2011).
